# Supplementary material for: Semilinear BSPDEs and Applications to McKean-Vlasov Control with Killing
Source: arXiv:2312.13468 source file (2023-12-20)
Supplement: Supplementary file 1 [file minimiser.tex]

\begin{lemma} \label{lem:minimiser}
Let $E_1$ and $E_2$ be complete separable metric spaces and let $G$ be a convex and closed subset of $\R^d$. Let $f \define E_1 \times E_2 \times G \to \R$ be a measurable map such that
\begin{enumerate}[noitemsep, label = (\roman*)]
    \item the map $g \mapsto f(x, y, g)$ is continuous for all $x \in E$;
    \item the map $g \mapsto f(x, y, g)$ is continuously differentiable for all $x \in E_1$, $y \in E_2$ and $\partial_g f$ is uniformly bounded;
    \item the map $g \mapsto f(x, y, g)$ is uniformly convex uniformly in $x \in E_1$, $y \in E_2$.
\end{enumerate}
Then there exists a measurable map $g_{\ast} \define E_1 \times E_2 \to G$ such that $y \mapsto g_{\ast}(x, y)$ is continuous for all $x \in E_1$ and $f(x, g_{\ast}(x)) = \inf_{g \in G}f(x, g)$ for all $x \in E_1$, $y \in E_2$.
\end{lemma}
